# Supplementary material for: Large zero-field cooled exchange-bias in bulk Mn2PtGa
Source: arXiv:1302.5229 source file (2013-02-21)
Supplement: Supplementary file 1 [file Supplementary_Mn2PtGa.pdf]

# Large zero-field-cooled exchange-bias in bulk $Mn_2PtGa$

## (Supplementary material)

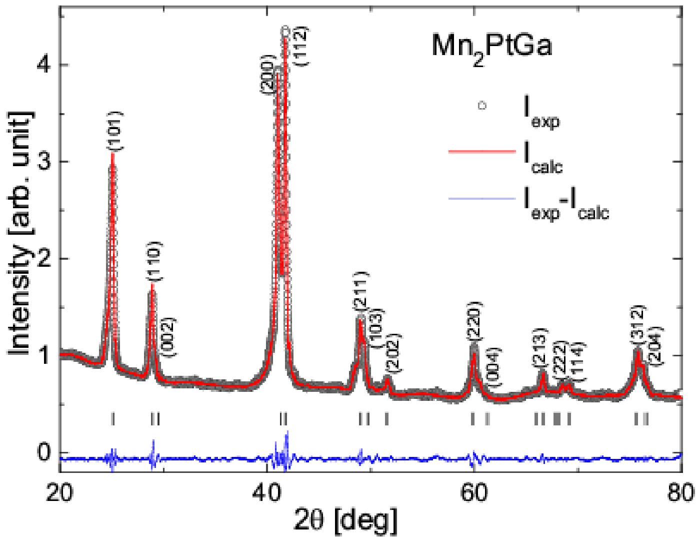


FIG. 1. Room temperature x-ray diffraction (XRD) pattern for $Mn_2PtGa$. The circles represent the experimental data, whereas, the red line corresponds to a simulation and the blue line shows the difference between the two curves.

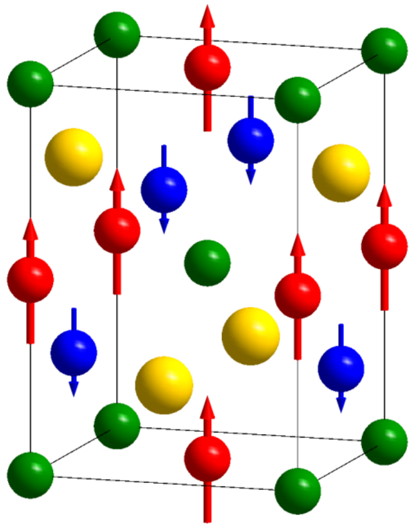

FIG. 2. Unit cell of the inverse tetragonal $Mn_2PtGa$ structure. The green spheres at the 2a position correspond to Ga, the red at the 2b position to Mn(I), the blue at the 2c position to Mn(II) and the golden at 2d position represent the Pt.

The room temperature XRD pattern for $Mn_2PtGa$ is shown in Fig. 1. To learn about the phase purity of the sample we have performed a Rietveld refinement using the space group I-4m2 that belongs to the inverse tetragonal structure. The refinement clearly shows that the sample is single phase. In the I-4m2 structure the Ga atoms occupy the 2a (0, 0, 0), the Mn(I) atoms the 2b (0, 0, 1/2), the Mn(II) atoms the 2c (0, 1/2, 1/4) and the Pt atoms the (0, 1/2, 1/4) Wyckoff positions. The refinement gives $a$=$b$=4.37 Å and $c$=6.05 Å. The tetragonal structure of the Heusler compounds mainly arises from the distortion of the cubic structure. The tetragonal distortion may occur in two ways: (i) elongation along the $c$ axis, (ii) contraction along the $c$ axis where $a$ remains same as in the cubic structure. The $c/a$ ratio of 1.38 ≈ $\sqrt{2}$ indicates that the tetragonal distortion in $Mn_2PtGa$ comes from the latter. As shown in Fig. 2, Mn(I) sitting at the octahedral position possesses a larger moment due to its localized nature. The Mn(II) sitting at the tetrahedral position, which possesses a smaller moment, align antiferromagnetically to the Mn(I). This configuration results in a ferrimagnetic structure with a net moment of around 0.55 $\mu_B$.

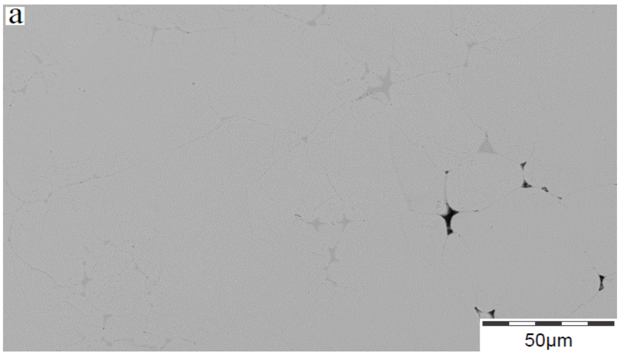

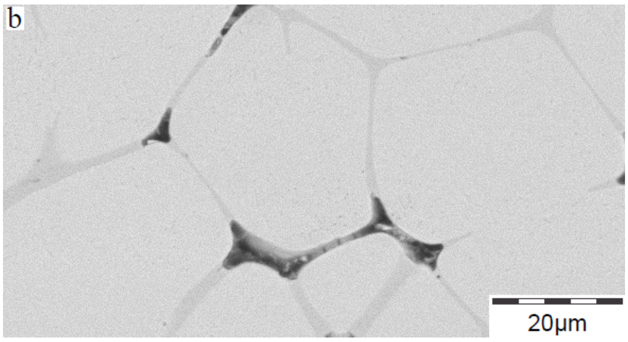


FIG. 3. (a) Scanning electron microscopy (SEM) image taken on the sample covering a larger area. (b) SEM image with higher magnification showing different grains.

Figure 3 shows an SEM images taken with different magnifications. It can be seen from FIG. 3a that the sample does not contain any secondary phase. To verify the nature of some dark gray lines and black spots observed in FIG. 3a, we have taken images with higher magnification as shown in FIG. 3b. From this we can easily see the formation of various grains. The dark gray lines observed in FIG. 3a and b mark the grain boundaries between the grains. We also observe several voids between grains which correspond to the black spots in FIG. 3a and b.
